# Supplementary material for: Search for variation of fundamental constants: Strong enhancements in $X^2\Pi$ cations of dihalogens and hydrogen halides
Source: arXiv:1502.04451 ancillary file (2015-02-16)
Supplement: Supplementary file 1 [file MS_2Pi_systems_Suppl.pdf]

# Supplementary Material
# Search for variation of fundamental constants: Strong enhancements in $X^2\Pi$ cations of dihalogens and hydrogen halides

L. F. Pašteka,[1,2,*] A. Borschevsky,[1,†] V. V. Flambaum,[3,1,‡] and P. Schwerdtfeger[1,§]

[1] *Centre for Theoretical Chemistry and Physics, The New Zealand Institute for Advanced Study, Massey University Auckland, Private Bag 102904, 0632 Auckland, New Zealand*
[2] *Department of Physical and Theoretical Chemistry, Faculty of Natural Sciences, Comenius University, Mlynská dolina, 84104 Bratislava, Slovakia*
[3] *School of Physics, University of New South Wales, Sydney 2052, Australia*

(Dated: February 9, 2015)

## I. SPECTROSCOPIC CONSTANTS

In the following we briefly define the symbols used in this work, following the definitions and the derivations of Ref. [1]. The energy of a vibrational-rotational level specified by the vibrational quantum number $\nu$, the total electronic angular momentum $J$, and its projection to the internuclear axis $\Omega$ ($\Omega = 1/2$ or $\Omega = 3/2$ for a molecule with a $^2\Pi$ ground state) is given by the Dunham series,

$$E_{\nu J\Omega} = G_\nu + F_J \pm \frac{A_\nu}{2}, \tag{1}$$

where $G_\nu$ is the energy of the vibrational level, $F_J$ is the energy of the rotational level, and $A_\nu$ is the spin-orbit coupling with the positive and the negative signs corresponding to $^2\Pi_{\frac{3}{2}}$ and $^2\Pi_{\frac{1}{2}}$ states, respectively. The energy of a given vibrational level is defined as a series in $(\nu + \frac{1}{2})$,

$$G_\nu = \omega_e(\nu + \frac{1}{2}) - \omega_e x_e(\nu + \frac{1}{2})^2 + \omega_e y_e(\nu + \frac{1}{2})^3 + \\ + \omega_e z_e(\nu + \frac{1}{2})^4 + \ldots \tag{2}$$

Similarly, the energy of a given rotational level is a series in $J(J+1)$,

$$F_J = B_\nu J(J+1) - D_\nu J^2(J+1)^2 + \ldots \tag{3}$$

The rotational constant $B_\nu$ and the centrifugal distortion constant $D_\nu$ depend on the vibrational quantum number $\nu$ and are given by

$$B_\nu = B_e - \alpha_e(\nu + \frac{1}{2}) + \gamma_e(\nu + \frac{1}{2})^2 + \epsilon_e(\nu + \frac{1}{2})^3 + \ldots \tag{4}$$

$$D_\nu = D_e + \beta_e(\nu + \frac{1}{2}) + \delta_e(\nu + \frac{1}{2})^2 + \ldots \tag{5}$$

The vibrationally dependent spin-orbit coupling constant $A_\nu$ is defined as

$$A_\nu = A_e + A^{(1)}(\nu + \frac{1}{2}) + A^{(2)}(\nu + \frac{1}{2})^2 + \ldots \tag{6}$$

and often the centrifugal distortion term $A_{D\nu}J(J+1)$ is added to the Eq. 6 as well, with

$$A_{D\nu} = A_D + A_D^{(1)}(\nu + \frac{1}{2}) + A_D^{(2)}(\nu + \frac{1}{2})^2 + \ldots \tag{7}$$

We note, that an extra term of $-B_\nu\Omega^2$ (giving raise to additional energy difference of $2B_\nu$ between the $^2\Pi_{\frac{3}{2}}$ and $^2\Pi_{\frac{1}{2}}$ sub-states) ought to be present in the expression for the rotational energy (3). In practice, however, this term is often effectively absorbed in the spin-orbit splitting (6). Only in the experimental works on $HBr^+$ and $HI^+$ this term was explicitly accounted for in the determination of the spectroscopic constants, hence we also include it only when reconstructing the energy levels of $HBr^+$ and $HI^+$ systems.

The collected experimental spectroscopic constants are summarised in Table I. Spectroscopic constants for $DI^+$ were obtained by isotopical scaling [2] from available experimental parameters for $HI^+$. We note, that the rotational constant $B_e$ and vibrational-rotational coupling constant $\alpha_e$ are given for the $^2\Pi_{\frac{3}{2}}$ sub-state of $I_2^+$ only [3], however we use them for both $^2\Pi_\Omega$ sub-states.

In cases where experimental spectroscopic constants $B_e$, $D_e$, and $\alpha_e$ are not given explicitly, we estimated these from the known constants by the use of simple relations. The rotational constant $B_e$ was calculated from the bond length $R_e$ and the reduced mass $M$ using the rigid-rotor relation,

$$B_e = \frac{\hbar}{4\pi c M R_e^2}. \tag{8}$$

For the centrifugal distortion constant $D_e$ the Kratzer formula [4] was assumed,

$$D_e = -\frac{4B_e^3}{\omega_e^2}. \tag{9}$$

Similarly, for the vibrational-rotational coupling constant $\alpha_e$ we used the Pekeris formula [5] derived from the

* lukas.f.pasteka@gmail.com
† a.borschevsky@massey.ac.nz
‡ v.flambaum@unsw.edu.au
§ p.a.schwerdtfeger@massey.ac.nz

TABLE I. Experimental spectroscopic constants (in cm$^{-1}$) of the systems under study. Asterisk denotes values calculated from other constants using Eqs. 8–10.

| | $H^{79}Br^+$ | $H^{81}Br^+$ | $D^{79}Br^+$ | $D^{81}Br^+$ | $HI^+$ | $^{79}Br_2^+$ | $^{79}Br^{81}Br^+$ | $^{81}Br_2^+$ | $I_2^+$ | $I^{79}Br^+$ | $I^{81}Br^+$ | $ICl^+$ | $IF^+$ |
|---|---|---|---|---|---|---|---|---|---|---|---|---|---|
| $\omega_e$ | 2439.8734 | 2439.4928 | 1736.786 | 1736.251 | 2195.243 | 365.5 | 363.05 | 360.85 | 234.5 | 301.5 | 300 | 433.1 | 691.5 |
| $\omega_e x_e$ | 46.1889 | 46.1740 | 23.3553 | 23.334 | 39.597 | 1.065 | 1.115 | 1.100 | 0.73 | 1.5 | 1.45 | 1.714 | 2.1 |
| $\omega_e y_e$ | 0.2304 | 0.2302 | 0.0828 | 0.0822 | | | | | | | | | |
| $\omega_e z_e \times 10^3$ | -1.92 | -1.90 | -0.34 | -0.29 | | | | | | | | | |
| $B_e$ | 8.07978 | 8.07715 | 4.09393 | 4.09145 | 6.33070 | 0.0886 | 0.0886 | 0.0886 | 0.03978 | 0.0610* | 0.0601* | 0.121* | 0.303* |
| $\alpha_e \times 10^3$ | 242.04 | 241.90 | 87.66 | 87.68 | 175.393 | 0.32 | 0.32 | 0.32 | 0.1182 | 0.376* | 0.355* | 0.795* | 2.25* |
| $\gamma_e \times 10^4$ | 9.56 | 9.45 | 2.9 | 3.34 | 1.6018 | | | | | | | | |
| $\epsilon_e \times 10^5$ | | | | | -6.616 | | | | | | | | |
| $D_e \times 10^6$ | 352.76 | 352.39 | 90 | 89 | 208.627 | 0.0208* | 0.0211* | 0.0214* | 0.00458* | 0.00999* | 0.00964* | 0.0376* | 0.233* |
| $\beta_e \times 10^6$ | -3.02 | -3.03 | | | -0.2710 | | | | | | | | |
| $A_e$ | -2652.663 | -2652.662 | -2652.35 | -2652.35 | -5359.2 | -2820 | -2820 | -2820 | -5197 | -4662 | -4662 | -4656.2 | -5690 |
| $A^{(1)}$ | 2.0609 | 2.0626 | 1.9 | 1.9 | 5.21137 | 5.0 | 3.7 | 3.9 | 11 | 3 | 0 | -8.1 | 9.0 |
| $A^{(2)}$ | 0.1597 | 0.1585 | | | | -0.11 | -0.03 | -0.06 | 0.04 | 1 | 1.1 | 0.734 | -1.8 |
| $A^{(3)}$ | 0.01051 | 0.01065 | | | | | | | | | | | |
| $A_D \times 10^4$ | 22.53 | 22.16 | | | 6.110 | -2 | -2 | -2 | | 2.41* | 2.37* | -0.541* | -13.2* |
| $A_D^{(1)} \times 10^4$ | 4.69 | 5.18 | | | 9.209 | 0.2 | 0.2 | 0.2 | | -0.0208* | -0.0196* | 0.00489* | 0.130* |
| $A_D^{(2)} \times 10^3$ | 9.66 | 9.09 | | | | | | | | | | | |

TABLE II. Experimental Λ-doubling parameters (in cm$^{-1}$)

| | $H^{79}Br^+$ | $H^{81}Br^+$ | $HI^+$ |
|---|---|---|---|
| $p_e$ | 2.0780 | 2.0846 | 3.52026 |
| $p^{(1)} \times 10^2$ | -2.68 | -2.64 | -4.9756 |
| $p^{(2)} \times 10^3$ | -1.29 | -1.35 | |
| $p_D \times 10^5$ | -6.23 | -5.66 | -9.403 |
| $p_D^{(1)} \times 10^6$ | -2.2 | -1.4 | |
| $q_e \times 10^3$ | -6.53 | -6.32 | -3.797 |
| $q^{(1)} \times 10^4$ | -9.5 | -9.9 | -2.552 |
| $q^{(2)} \times 10^4$ | 1.40 | 1.56 | |

Morse potential,

$$\alpha_e = \frac{6B_e^2}{\omega_e}\left(\frac{\omega_e x_e}{\sqrt{B_e}} - 1\right). \quad (10)$$

Expressions (8) – (10) were used for estimation of $B_e$, $D_e$, and $\alpha_e$ for systems $IF^+$, $ICl^+$, and $IBr^+$. In the case of $IF^+$ the bond lengths were experimental ($R_e = 1.836$ and 1.832 Å for $^2\Pi_{\frac{3}{2}}$ and $^2\Pi_{\frac{1}{2}}$, respectively [6]), and for $ICl^+$ and $IBr^+$ we computed the bond lengths using the DIRAC13 program package [7] through a fully relativistic four-component Fock-space coupled cluster (4c-FS-CCSD) method [8] with aug-cc-pVQZ basis sets [9, 10] for Cl and Br and a Faegri dual basis set [11] for I. The resulting values used in this work are $R_e(^2\Pi_{\frac{3}{2}}) = 2.233$ Å, $R_e(^2\Pi_{\frac{1}{2}}) = 2.232$ Å for $ICl^+$ and $R_e(^2\Pi_{\frac{3}{2}}) = 2.381$ Å, $R_e(^2\Pi_{\frac{1}{2}}) = 2.385$ Å for $IBr^+$.

Effect of Λ-doubling further splits the doubly degenerate rotational $^2\Pi_\Omega$ levels by a small energy difference, given as

$$\Delta E_{ef}(^2\Pi_{\frac{1}{2}}) = (p_\nu + 2q_\nu)(J + \frac{1}{2}), \quad (11)$$

$$\Delta E_{ef}(^2\Pi_{\frac{3}{2}}) = (\frac{p_\nu}{Y_\nu^2} + \frac{2q_\nu}{Y_\nu})(J - \frac{1}{2})(J + \frac{1}{2})(J + \frac{3}{2}) \quad (12)$$

with $Y_\nu = A_\nu/B_\nu$ and the Λ-doubling parameters $p_\nu$ and $q_\nu$ having vibrational dependence analogous to Eq. 6 and usually also the centrifugal distorsion analogous to Eq. 7. The split levels are labeled $e/f$ according to their rotational symmetry in the non-alternating fashion (as opposed to the $+/-$ labels) [12].

In the case of $HBr^+$ and $HI^+$ the Λ-doubling was resolved and described by experiment [13, 14] and resulting experimental constants are given in Table II. Parameters for the deuterated isotopologues were obtained by isotopical scaling [2].

For the studied dihalogen cations Λ-doubling was not observed in the experiment, since the resolution was not high enough. Hence we calculated the Λ-doubling parameters assuming the pure precession approximation (PPA) [15, 16] as

$$p_\nu = \frac{4A_\nu B_\nu}{\Delta E_{\Sigma\Pi}}, \quad q_\nu = \frac{4B_\nu^2}{\Delta E_{\Sigma\Pi}}, \quad (13)$$

where $\Delta E_{\Sigma\Pi}$ is the energy difference between the $X^2\Pi$ ground state and the nearest excited $^2\Sigma$ state, which accounts for majority of the interaction.

For the closely related dihalogen $Cl_2^+$ the Λ-doubling parameters $p_1$ and $p_2$ were determined by experiment [17] to have values 0.0202 and 0.0200 cm$^{-1}$, respectively. These are reasonably well reproduced by the PPA expressions (13) with the corresponding values of –0.0226 and –0.0225 cm$^{-1}$ (note that the sign only dictates the correct order of +/− or $e/f$ rotational symmetry levels, which were not assigned in the experiment). This justifies the use of the PPA for the studied dihalogen cations. The $B^2\Sigma^+_{(g)}$ excitation energies were determined using the DIRAC13 program package [7] using the FS-CCSD method with the Dyall's v3z basis set [18, 19] in the exact two-component (X2C) formalism [20, 21]. Resulting energies reproduce well the experimental values reported in Refs. [22, 23], relative errors being less than 4% in all cases. We used the experimental excitation energies in Eq. 13 for $Br_2^+$ and $I_2^+$ and the theoretical values for $IBr^+$, $ICl^+$ (for which the exerimental values were to some extent estimated), and $IF^+$ (for which no experimental value was available).

## II. OTHER MOLECULES CONSIDERED

For the sake of completeness we briefly mention the remaining systems belonging to the group of cations of dihalogens and hydrogen halides. $ClF^+$, $BrF^+$, and $BrCl^+$ were studied by low-resolution He(I) photoelectron spectroscopy and a few basic spectroscopic constants are given in the corresponding works [24–26]. However, because of the considerable uncertainties in the values, we cannot use these for our analysis. For $ClF^+$ only the harmonic vibrational frequency $\omega_e = 870 \pm 30$ cm$^{-1}$ and the spin-orbit coupling constant $A_e = -630 \pm 30$ cm$^{-1}$ are reported [24]. Since the value of $A_e$ is smaller than that of $\omega_e$, this renders $ClF^+$ unfavourable for observing quasi-degeneracies between vibrational levels of the $^2\Pi_{\frac{3}{2}}$ and $^2\Pi_{\frac{1}{2}}$ substates. Only with sufficiently large negative $A^{(1)}$ constant, quasi-degeneracy could occur for some higher vibrational levels, but this is unlikely considering the fact that we do not observe this in the related systems $F_2^+$ and $Cl_2^+$ (discussed below). In the case of $BrF^+$, three spectroscopic constants are reported, namely $\omega_e = 750 \pm 30$ cm$^{-1}$, $\omega_e x_e = 10 \pm 5$ cm$^{-1}$, and $A_e = -2590 \pm 40$ cm$^{-1}$ [25]. Depending on the value of $A^{(1)}$, this system might exhibit quasi-degeneracies similar to the $IF^+$ cation, but we cannot draw any further conclusions from the present values. The $BrCl^+$ cation seems to be the most promising of these three systems with the reported values $\omega_e = 498 \pm 20$ cm$^{-1}$, $\omega_e x_e = 2.5 \pm 5.0$ cm$^{-1}$, $A_e = -2070 \pm 30$ cm$^{-1}$, and $A^{(1)} = -24 \pm 20$ cm$^{-1}$ [26]. Since the spin-orbit coupling constant is approximately four times the harmonic vibrational frequency, there is a possibility of quasi-degeneracy between the $^2\Pi_{\frac{3}{2}}(\nu = 4)$ and $^2\Pi_{\frac{1}{2}}(\nu = 0)$ levels. The energies corresponding to these levels (with respect to the bottom of the $^2\Pi_{\frac{3}{2}}$ potential well) are 2140 ± 160 cm$^{-1}$ and 2320 ± 40 cm$^{-1}$, respectively, showing a slight overlap between the two uncertainty intervals. Similar situation holds for several higher vibrational levels.

The $HF^+$, $HCl^+$, and $F_2^+$ cations were studied extensively by experiment and their spectroscopic constants are known to high precision. However, since the spin-orbit coupling constant is much smaller than the vibrational frequency ($A_e = -292.6$ cm$^{-1}$, $\omega_e = 3097.1$ cm$^{-1}$ for $HF^+$ [27], $A_e = -648.3$ cm$^{-1}$, $\omega_e = 2673.7$ cm$^{-1}$ for $H^{35}Cl^+$ [28], and $A_e = -337$ cm$^{-1}$, $\omega_e = 1089.4$ cm$^{-1}$ for $F_2^+$ [29]), no quasi-degeneracy between the $X^2\Pi$ substates is observed throughout the whole region of vibrational levels. Similar situation holds for the deuterated species $DF^+$ and $DCl^+$. This is nicely illustrated for all three cations in the spectra in Refs. [30–32].

Although $Cl_2^+$ was previously suggested as a good candidate for VFC study [33] based on spectroscopic constants from Ref. [34], recent data from high-resolution spectroscopy [35] revealed that the match between the spin-orbit coupling constant and the vibrational frequency is not as fortuitous as expected. The corresponding values from this study are $A_e = -717.5$ cm$^{-1}$ and $\omega_e = 645.6$ cm$^{-1}$ for $^{35}Cl_2^+$. Since the $^2\Pi_{g,\frac{1}{2}}(\nu = 0)$ level is above the $^2\Pi_{g,\frac{3}{2}}(\nu = 1)$ level, and the vibrational dependence of the spin-orbit term $A_v$ is negligible, every subsequent pair of levels is even further apart in energy because of the effect of anharmonicity. The smallest energy difference of 59.5 cm$^{-1}$ between levels $X^2\Pi_{g,\frac{1}{2}}$, $\nu = 0$ and $X^2\Pi_{g,\frac{3}{2}}$, $\nu = 1$ can be observed for the $^{37}Cl_2^+$ isotopologue; however, this is still too large. The value of the rotational constant $B_e$ is approximately 0.28 cm$^{-1}$, hence no further improvement can be obtained for any rotational levels. Nevertheless, the $Cl_2^+$ is still an interesting system with many quasi-degeneracies between the vibrational levels of the ground state $X^2\Pi_g$ and excited states $A^2\Pi_u$, $B^2\Delta_u$, and $a^4\Sigma_u^-$, which we investigate in a separate study.

## III. MOLECULAR ENERGY LEVELS

Following figures depict the potential energy curves for the substates of $X^2\Pi$ ground state with selected quasi-degeneracies between vibrational levels in the systems of study (Fig. 1) and the respective rotational structure of these levels with several favourable transitions (Fig. 2).

The potential energy curves and vibrational levels of the two respective isotopologues of systems $ICl^+$, $HBr^+$, and $DBr^+$ (differing only in the Br or Cl isotope) are indistinguishable from one another within the scope of Fig. 1. Similarly, the rotational levels of the two respective isotopologues of $HBr^+$ and $DBr^+$ are qualitatively identical, hence we ommit the rotational plots for $H^{81}Br^+$ and $D^{81}Br^+$ in Fig. 2.

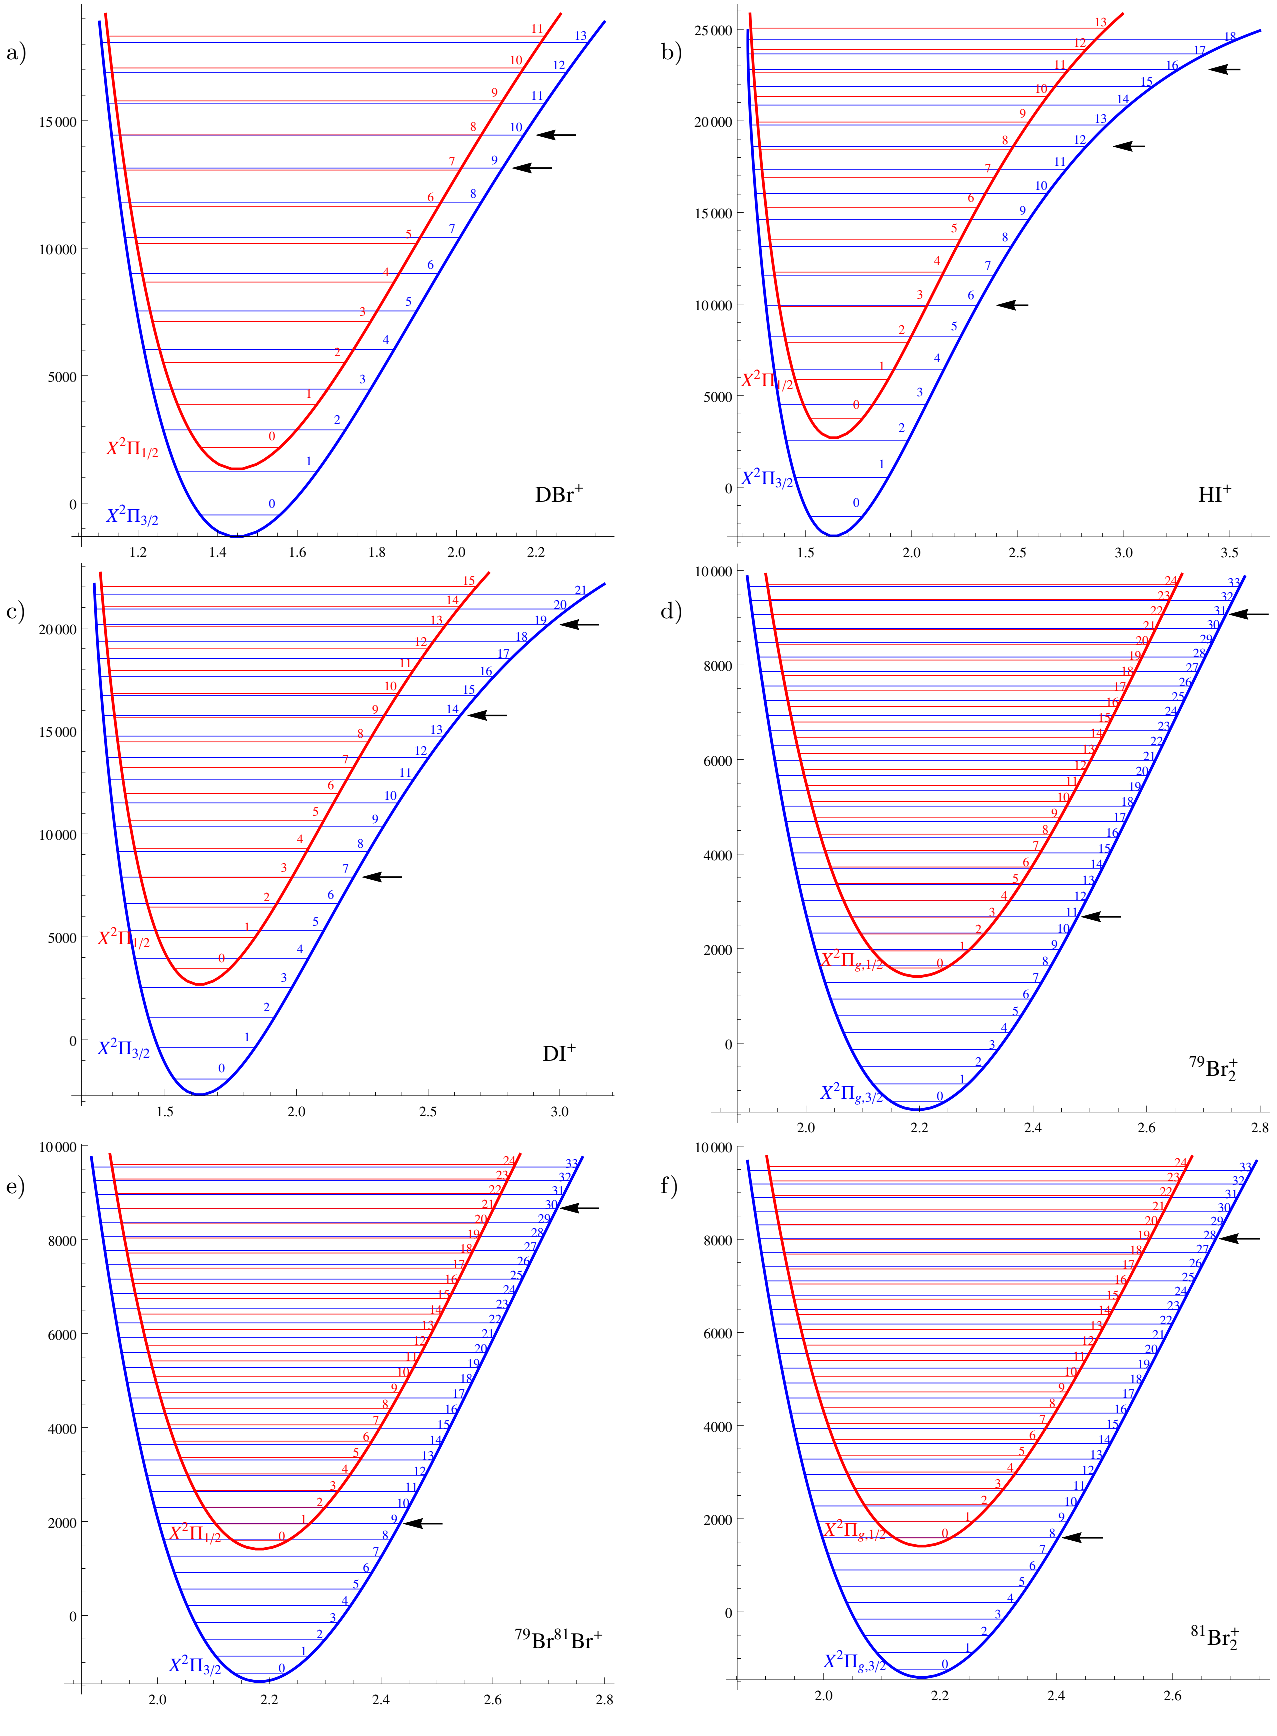


FIG. 1. Potential energy curves of a) $DBr^+$, b) $HI^+$, c) $DI^+$, d) $^{79}Br_2^+$, e) $^{79}Br^{81}Br^+$, f) $^{81}Br_2^+$, g) $I_2^+$, h) $I^{79}Br^+$, i) $I^{81}Br^+$, i) $ICl^+$, and j) $IF^+$. The arrows point to the quasi-degenerate vibrational levels of the two substates of the $X^2\Pi$ state. (*continues on the following page*)

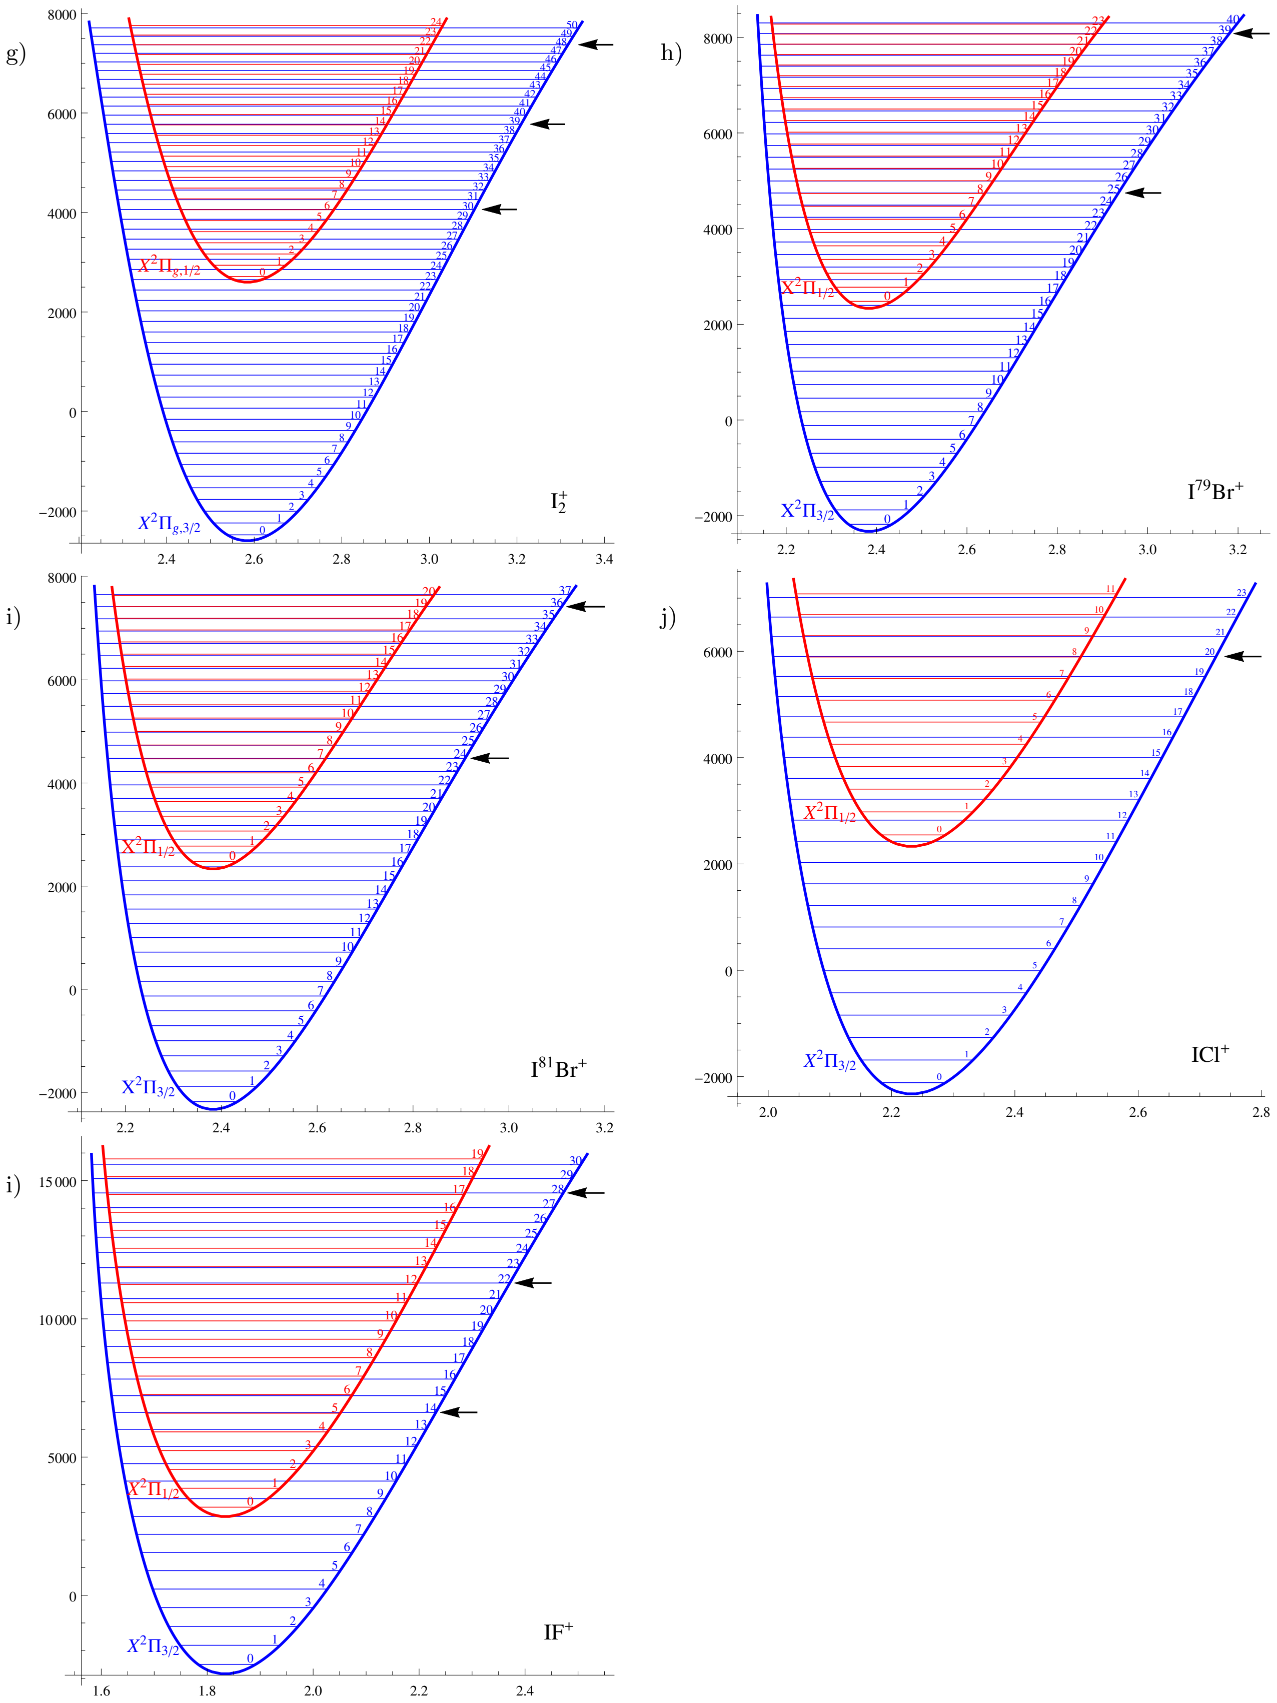


FIG. 1. (*continued*)

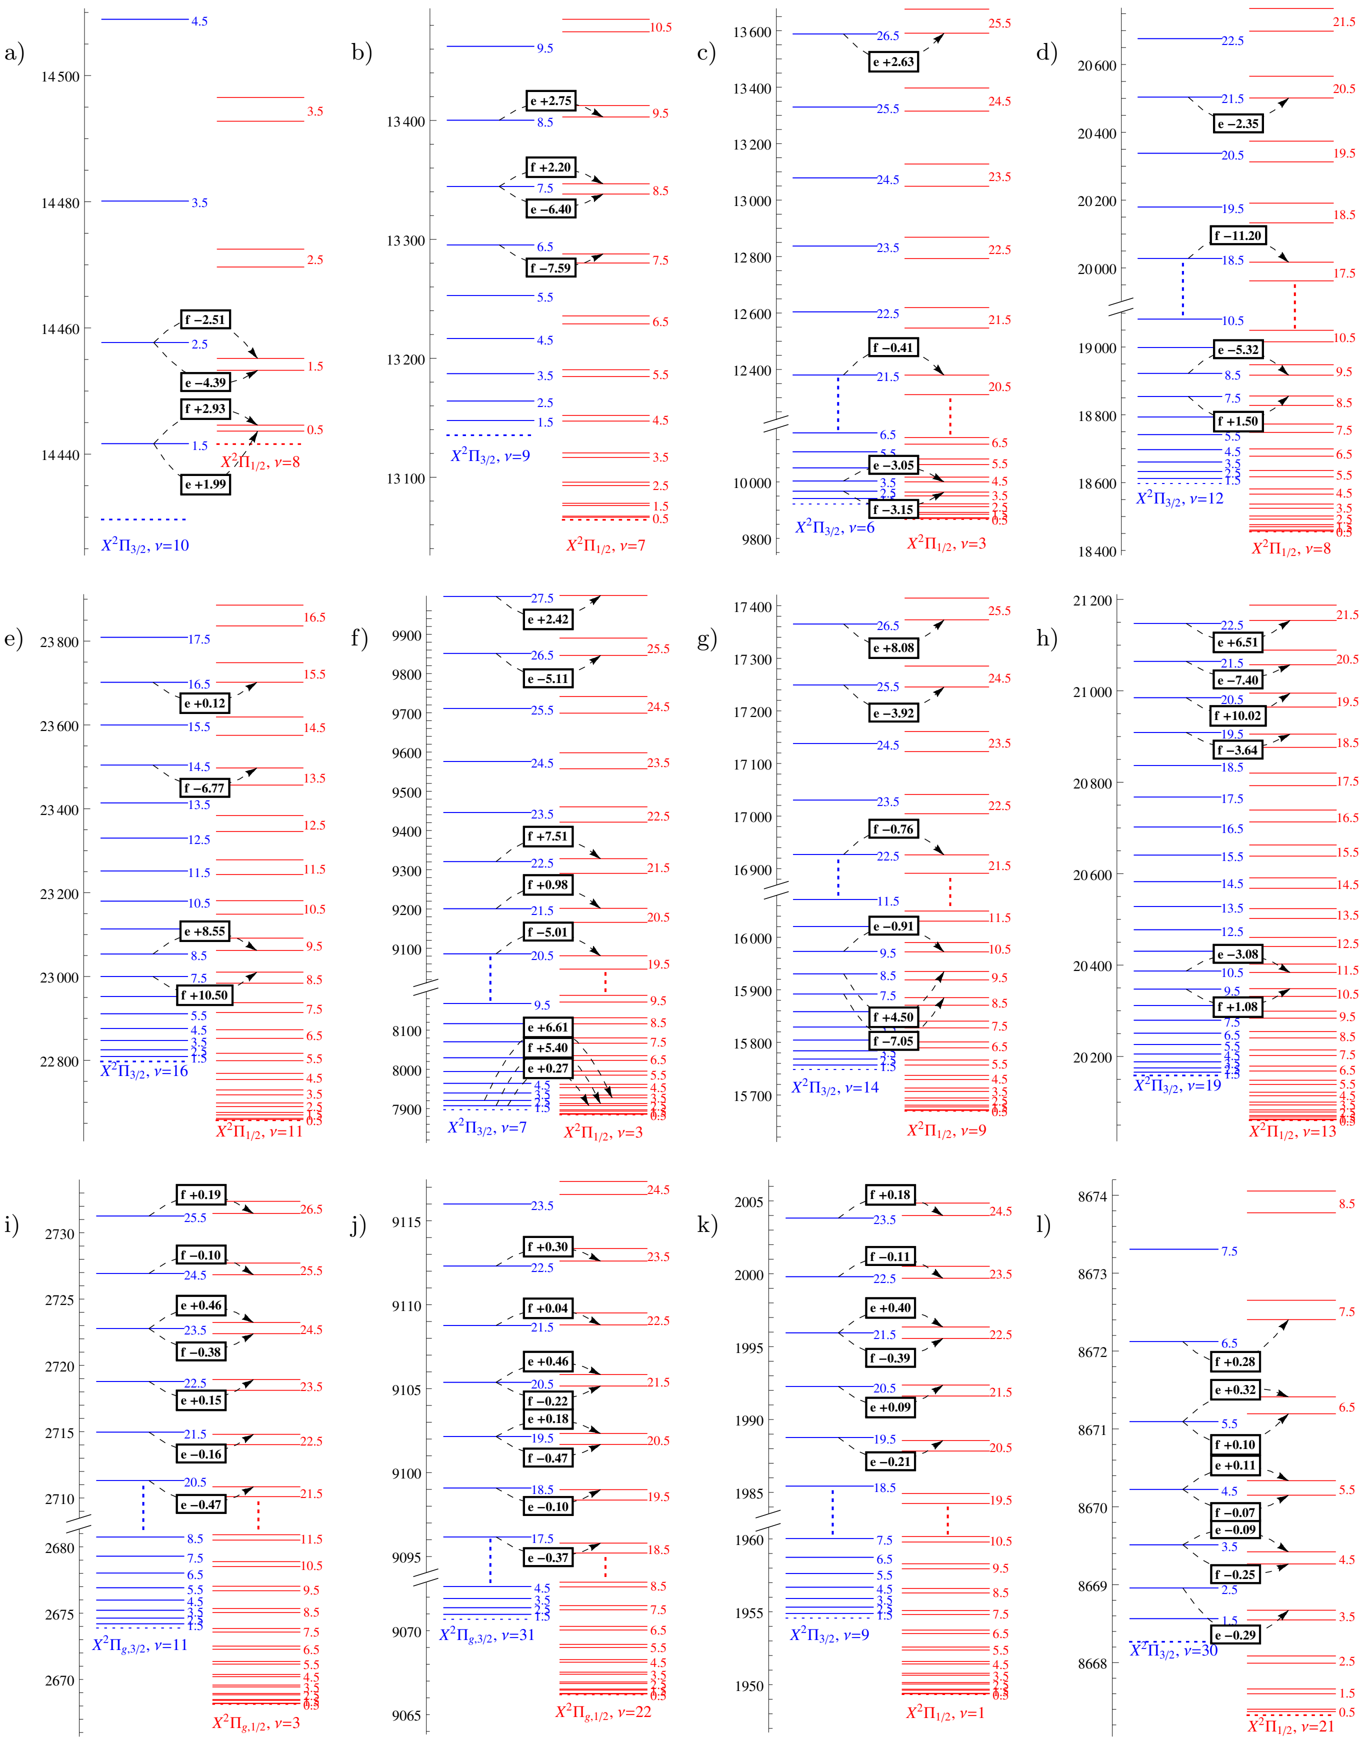


FIG. 2. Rotational structure of the selected quasi-degenerate vibrational levels of the two $X^2\Pi$ substates of a–b) $D^{79}Br^+$, c–e) $HI^+$, f–h) $DI^+$, i–j) $^{79}Br_2^+$, k–l) $^{79}Br^{81}Br^+$, m–n) $^{81}Br_2^+$, o–q) $I_2^+$, r) $I^{35}Cl^+$, s) $I^{37}Cl^+$, t–u) $I^{79}Br^+$, v–w) $I^{81}Br^+$, and x–z) $IF^+$ with transition energies in $cm^{-1}$. Allowed $e \leftrightarrow e$ and $f \leftrightarrow f$ transitions are denoted with $e$ and $f$, respectively, in the brackets with transition energies. (*continues on the following page*)

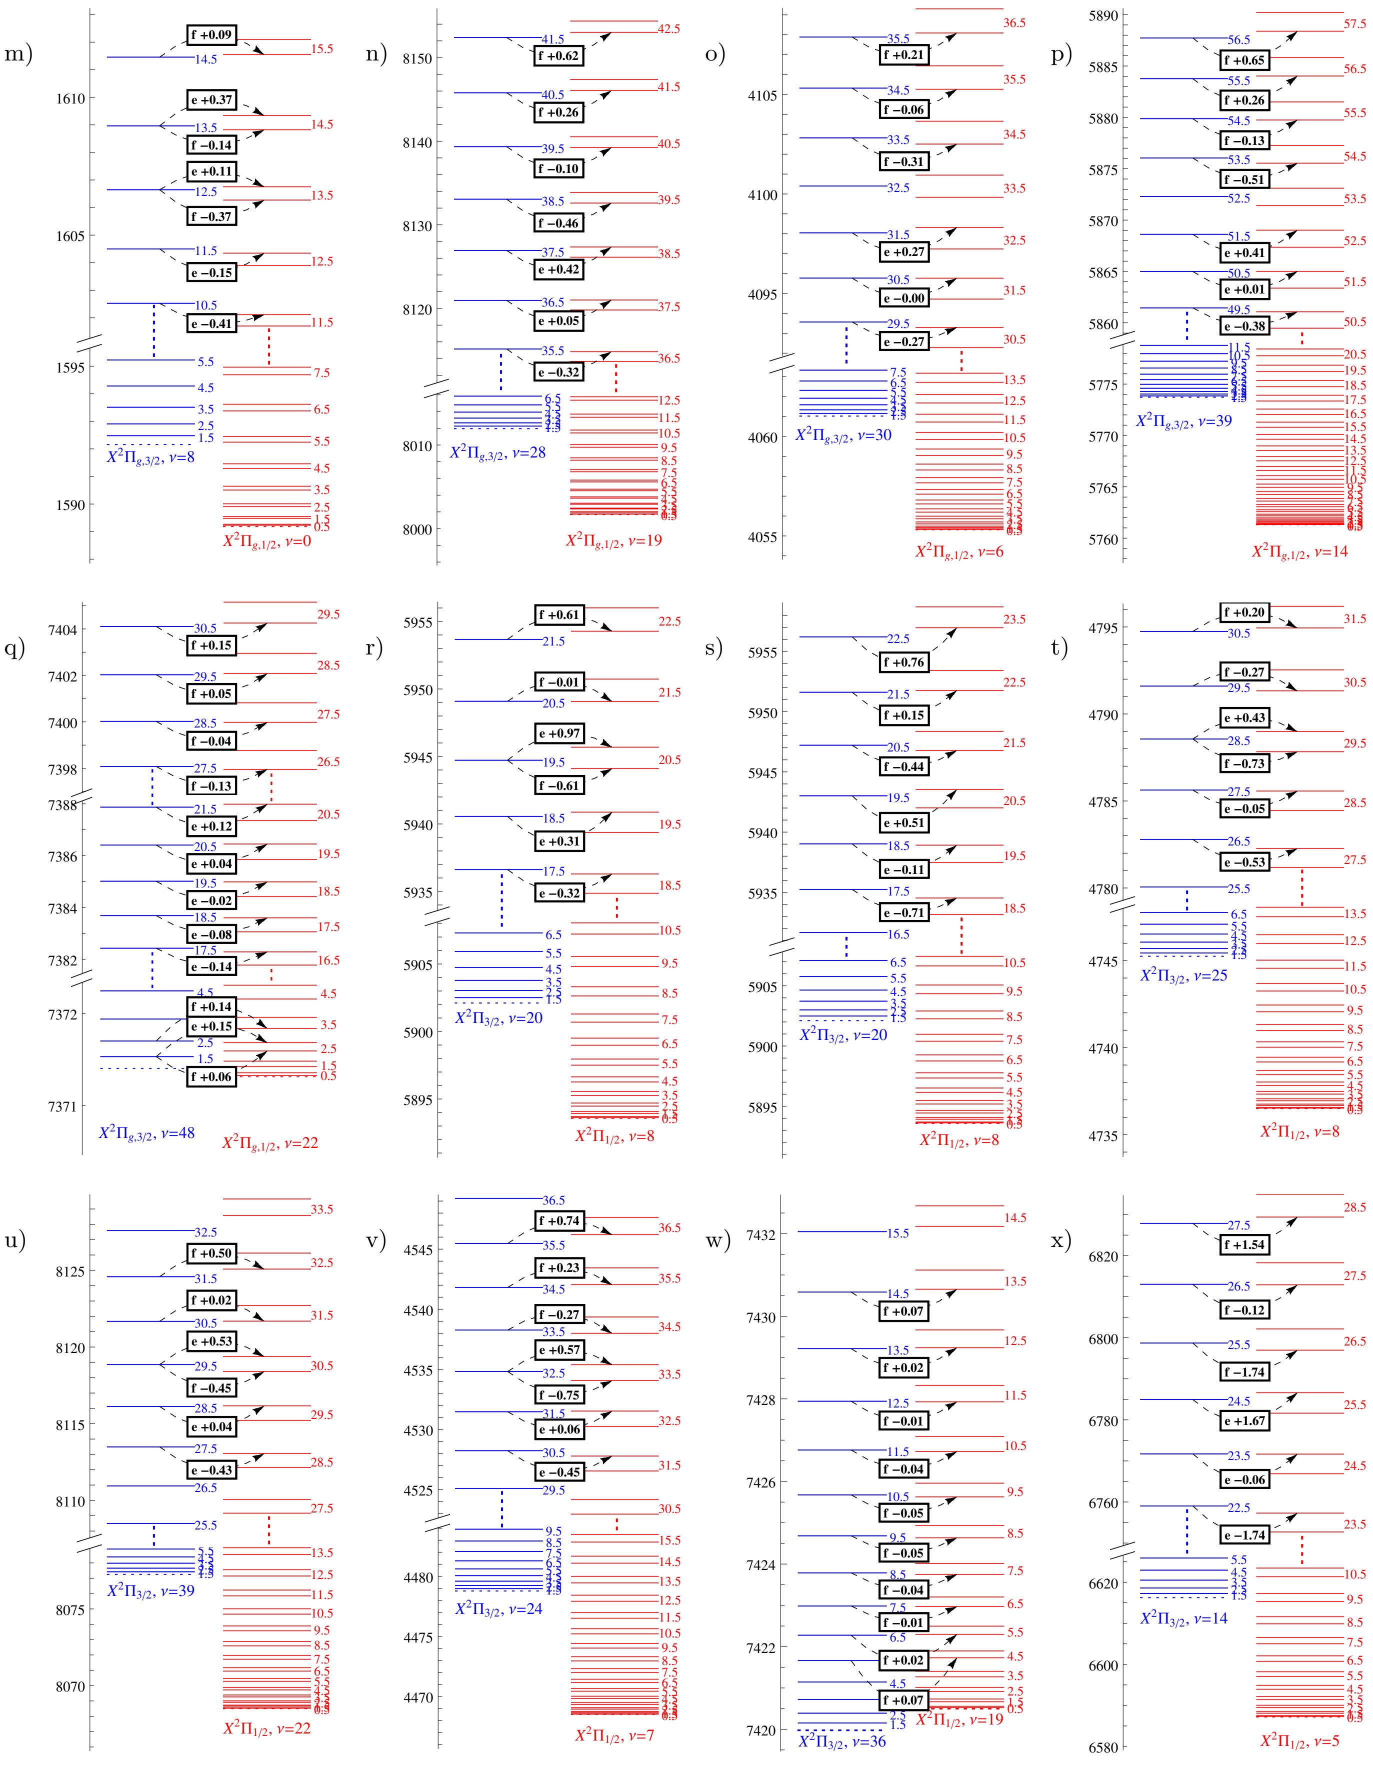


FIG. 2. (*continued*)

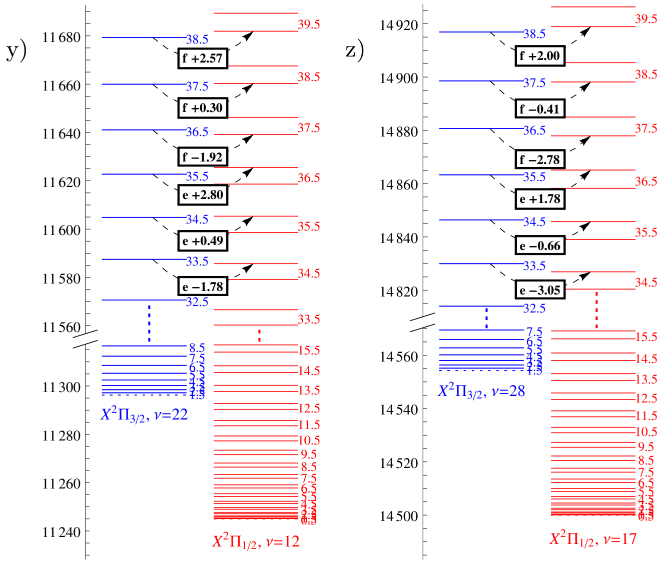


FIG. 2. (*continued*)


[1] H. Lefebvre-Brion and R. Field, in *The Spectra and Dynamics of Diatomic Molecules* (Elsevier, 2004).

[2] R. Mulliken, Phys. Rev. **25**, 119 (1925).

[3] L.-h. Deng, Y.-y. Zhu, C.-l. Li, and Y.-q. Chen, J. Chem. Phys. **137**, 054308 (2012).

[4] A. Kratzer, Z. Phys. **3**, 289 (1920).

[5] C. Pekeris, Phys. Rev. **45**, 98 (1934).

[6] F. Innocenti, M. Eypper, S. Beccaceci, A. Morris, S. Stranges, J. B. West, G. C. King, and J. M. Dyke, J. Phys. Chem. A **112**, 6939 (2008).

[7] DIRAC, a relativistic ab initio electronic structure program, Release DIRAC13 (2013), written by L. Visscher, H. J. Aa. Jensen, R. Bast, and T. Saue, with contributions from V. Bakken, K. G. Dyall, S. Dubillard, U. Ekström, E. Eliav, T. Enevoldsen, E. Faßhauer, T. Fleig, O. Fossgaard, A. S. P. Gomes, T. Helgaker, J. K. Lærdahl, Y. S. Lee, J. Henriksson, M. Iliaš, Ch. R. Jacob, S. Knecht, S. Komorovský, O. Kullie, C. V. Larsen, H. S. Nataraj, P. Norman, G. Olejniczak, J. Olsen, Y. C. Park, J. K. Pedersen, M. Pernpointner, K. Ruud, P. Sałek, B. Schimmelpfennig, J. Sikkema, A. J. Thorvaldsen, J. Thyssen, J. van Stralen, S. Villaume, O. Visser, T. Winther, and S. Yamamoto (see http://www.diracprogram.org).

[8] L. Visscher, E. Eliav, and U. Kaldor, J. Chem. Phys. **115**, 9720 (2001).

[9] D. E. Woon and T. H. Dunning, J. Chem. Phys. **98**, 1358 (1993).

[10] A. K. Wilson, D. E. Woon, K. A. Peterson, and T. H. Dunning, J. Chem. Phys. **110**, 7667 (1999).

[11] K. Faegri, Theor. Chim. Acta **105**, 252 (2001).

[12] J. Brown and A. Carrington, *Rotational Spectroscopy of Diatomic Molecules*, Cambridge Molecular Science (Cambridge University Press, 2003).

[13] A. Chanda, W. C. Ho, F. W. Dalby, and I. Ozier, J. Chem. Phys. **102**, 8725 (1995).

[14] A. Chanda, W. Ho, F. Dalby, and I. Ozier, J. Mol. Spectrosc. **169**, 108 (1995).

[15] J. H. Van Vleck, Phys. Rev. **33**, 467 (1929).

[16] R. S. Mulliken and A. Christy, Phys. Rev. **38**, 87 (1931).

[17] J. Choi and J. Hardwick, Journal of Molecular Spectroscopy **137**, 138 (1989).

[18] K. G. Dyall, Theoretical Chemistry Accounts **108**, 335 (2002).

[19] K. Dyall, Theoretical Chemistry Accounts **115**, 441 (2006).

[20] K. G. Dyall, The Journal of Chemical Physics **106**, 9618 (1997).

[21] T. Saue, ChemPhysChem **12**, 3077 (2011).

[22] H. V. Lonkhuyzen and C. D. Lange, Chemical Physics **89**, 313 (1984).

[23] R. Tuckett, E. Castellucci, M. Bonneau, G. Dujardin, and S. Leach, Chemical Physics **92**, 43 (1985).

[24] R. DeKock, B. Higginson, D. Lloyd, A. Breeze, D. Cruckshank, and D. Armstrong, Mol. Phys. **24**, 1059 (1972).

[25] E. Colbourn, J. Dyke, N. Fayad, and A. Morris, J. Electron Spectr. Related Phen. **14**, 443 (1978).

[26] S. Dunlavey, J. Dyke, and A. Morris, J. Electron Spectr. Related Phen. **12**, 259 (1977).

[27] P. C. Cosby, H. Helm, and M. Larzilliere, J. Chem. Phys. **94**, 92 (1991).

[28] J. M. Brown and J. K. G. Watson, J. Mol. Spect. **65**, 65 (1977).

[29] R. Tuckett, A. Dale, D. Jaffey, P. Jarrett, and T. Kelly, Mol. Phys. **49**, 475 (1983).

[30] A. J. Yencha, A. J. Cormack, R. J. Donovan, A. Hopkirk, and G. C. King, J. Phys. B: At. Mol. Opt. Phys. **32**, 2539 (1999).

[31] A. Yencha, A. Cormack, R. Donovan, A. Hopkirk, and G. King, Chem. Phys. **238**, 109 (1998).

[32] A. Cormack, A. Yencha, R. Donovan, K. Lawley, A. Hopkirk, and G. King, Chem. Phys. **213**, 439 (1996).

[33] V. Flambaum and M. Kozlov, "Studying variation of fundamental constants with molecules," in *Cold Molecules:*

*Theory, Experiment, Applications*, edited by R. V. Krems, W. C. Stwalley, and B. Friedrich (CRC Press, 2009) p. 451.

[34] K. Huber and G. Herzberg, in *NIST Chemistry WebBook*, NIST Standard Reference Database No. 69, edited by P. Linstrom and W. Mallard (National Institute of Standards and Technology, Gaithersburg MD, 2011) http://webbook.nist.gov.

[35] S. Mollet and F. Merkt, J. Chem. Phys. **139**, 034302 (2013).
